# Supplementary material for: Observing quantum state diffusion by heterodyne detection of fluorescence
Source: arXiv:1511.01415 ancillary file (2015-11-04)
Supplement: Supplementary file 1 [file supplementary-materials.pdf]

# Supplementary Materials for

# "Observing quantum state diffusion by heterodyne detection of fluorescence"

P. Campagne-Ibarcq,[1,2] P. Six,[3,2] L. Bretheau,[1,2] A. Sarlette,[2] M. Mirrahimi,[2] P. Rouchon,[3,2] and B. Huard[1,2]

[1]*Laboratoire Pierre Aigrain, Ecole Normale Supérieure-PSL Research University, CNRS, Université Pierre et Marie Curie-Sorbonne Universités, Université Paris Diderot-Sorbonne Paris Cité, 24 rue Lhomond, 75231 Paris Cedex 05, France*
[2]*Quantic Team, INRIA Paris-Rocquencourt, Domaine de Voluceau, B.P. 105, 78153 Le Chesnay Cedex, France*
[3]*Centre Automatique et Systèmes, Mines ParisTech, PSL Research University, 60 Boulevard Saint-Michel, 75272 Paris Cedex 6, France.*
(Dated: November 4, 2015)

## I. MATERIAL AND METHODS

### A. Sample fabrication and characterization

The superconducting qubit follows the design of the "3D transmon" described in Ref. [1]. A single aluminum Josephson junction connected to two antennas of $0.4 \times 1$ mm$^2$ each is embedded in a copper cavity of $26.5 \times 26.5 \times 9.5$ mm$^3$, anchored at the base-temperature (20 mK) of a dilution refrigerator. The transmon chip was fabricated on a single-crystal C-plane sapphire substrate, using electron-beam lithography followed by double-angle electron-beam evaporation of aluminum. Film thickness for each evaporation is approximately 30 nm and 85 nm which takes into account the evaporation angles $\pm 30$Â°. The two layers are separated by a thin AlOx layer grown in an atmosphere of 20 % $O_2$ and 80 % Ar at 20 mbar for 7 min to form the tunnel junction. The room temperature resistance of the junction was measured to be 3.2 k$\Omega$.

With these parameters, the qubit resonates at $f_q = 6.37$ GHz and is dispersively coupled to the cavity first resonant mode at $f_c = 7.8$ GHz. The full system hamiltonian then reads

$$H = hf_c a^\dagger a + hf_q \frac{\sigma_z}{2} - h\chi a^\dagger a \frac{\sigma_z}{2}, \tag{S1}$$

where the cavity pull is measured to be $\chi = 11.5$ MHz.
The cavity mode is coupled to two transmission lines (Fig. S1). The coupling to the output line on which the detection of the fluorescence is performed is much larger than the one to the input line and than the cavity internal losses. From continuous wave transmission and reflection measurement on the cavity ports, we extract the photon exit rate at cavity frequency through the output port of $\kappa_{\mathrm{out}} = 2\pi \times 3$ MHz. The total photon exit rate is $\kappa_{\mathrm{tot}} = 2\pi \times 3.45$ MHz.

From the same measurements, we estimate the occupation of the excited state of the qubit $p_{\mathrm{eq}}(|e\rangle) = 0.7\ \% \pm 0.3\ \%$, corresponding to an effective temperature $T_q = 60$ mK (see Fig. S2). Note that the cavity surface was etched at room temperature in highly concentrated hydrochloric acid (HCl, 37%) for about 1 min before the experiment. The same sample (same chip, same cavity and similar coupling rates to the probe lines) was characterized in a previous run before surface etching, and the occupation of the excited state at thermal equilibrium was then measured to be $\tilde{p}_{\mathrm{eq}}(|e\rangle) = 7\ \% \pm 0.5\ \%$.

### B. Measurement setup

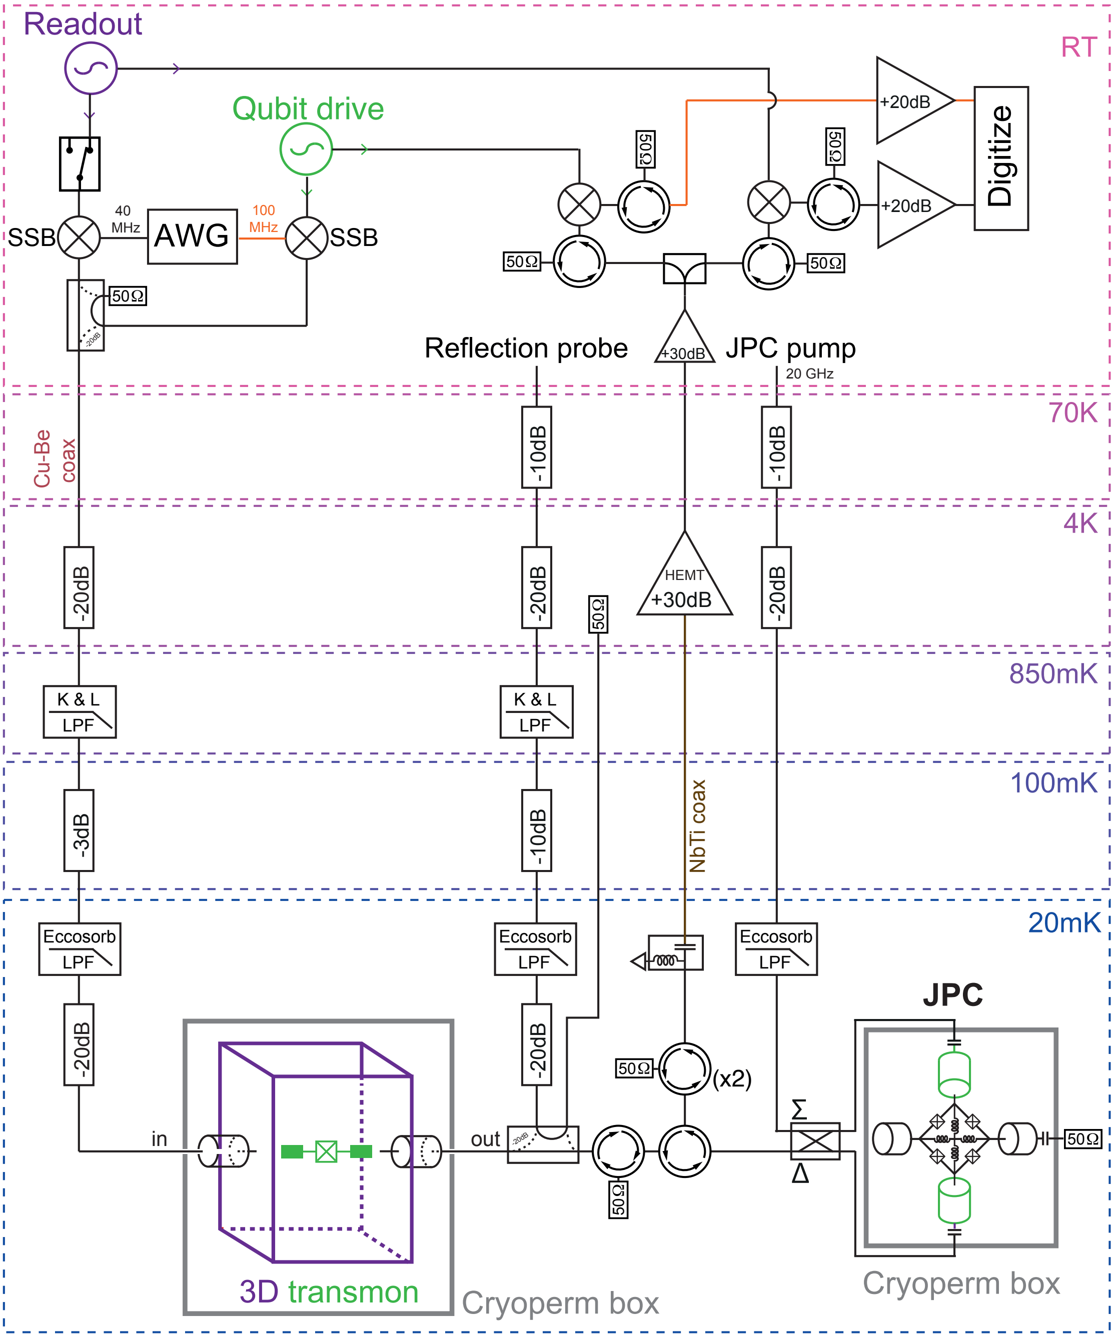


Figure S1: **Schematics of the experimental setup.** Readout and qubit rotation pulses are generated by single side-band (SSB) modulation and sent through the input line, which is heavily attenuated (XMA attenuators) and filtered (K&L and homemade Eccosorb low-pass filters (LPF)). The fluorescence field from the qubit on the output line is amplified by a Josephson Parametric Converter (JPC) and routed out of the fridge. The same source used to generate preparation pulses of the qubit is used to down convert the resulting signal to 100 MHz (in orange) before digitization and numerical demodulation.

Figure S1 is a block diagram of the measurement setup. The system is probed through SMA connectors whose central pin dips inside the 3D cavity. Readout and rotation pulses on the qubit are generated by standard single side-band (SSB) modulation of continuous microwave tones. The modulation is performed by mixing on a commercial SSB modulator by PolyphaseMicrowave the continuous waves produced by microwave generators with pulsed sinusoidal signals synthesized by different channels of a Tektronix Arbitrary Waveform Generator (AWG). All sources are synchronized by a shared atomic clock.

These pulses are sent through a heavily attenuated and filtered input coax line (with cryogenic attenuators at various stages of the dilution refrigerator), ensuring that negligible thermal excitations enter the device. A commercial low-pass filter (from K&L) with 12 GHz cut-off frequency is used at the still stage (850 mK), while a homemade low-pass filter consisting in a microstrip line enclosed in an infrared tight box filled with Eccosorb is inserted at base temperature. Note that a similar line, denoted as "reflection probe" in Fig. S1, is used for an in situ calibration of the cavity ouput coupling rates $\kappa_{out}$ (see subsection I A), but is unused in the discussed experiment. Finally, the copper cavity is enclosed in a cryoperm shield and anchored at the 20 mK stage of the refrigerator. An aluminum foil is wrapped around the cavity to screen residual magnetic fields using the Meissner effect.

Two cryogenic circulators in series are used to direct the fluorescence field on the output line from the cavity toward a Josephson Parametric Converter [2] (JPC), which is here used as a low noise non-degenerate amplifier at qubit frequency $f_q$. It is pumped with a continuous pump tone at 18 GHz and realizes a +25 dB gain with 3 MHz bandwidth. A cryoperm magnetic shield encloses the JPC and its biasing coil (not shown). The output signal of the JPC is routed back through a superconducting NbTi coax cable towards a low noise HEMT (High Electron Mobility Transistor) amplifier with 30 dB of gain from Caltech University. It is isolated with two circulators in series and the inner cable is thermalized using a bias-tee anchored at base temperature. The signal is further amplified at room temperature and down-converted to 100 MHz before being digitized at 500 MS.s$^{-1}$ and numerically demodulated by an ATS9351 Alazar board.

The readout pulses at cavity frequency are transmitted to the output line, reflected on the JPC (gain unity) and routed out of the refrigerator on the same line as the fluorescence signal. They are then down converted to 40 MHz and digitized on a second ADC of the Alazar board. A fast RF switch is placed on the readout input line in order to better isolate the qubit from Local Oscillator leakage close to the cavity resonance frequency, which would otherwise degrade the qubit coherence time.

### C. Projective readout of the qubit

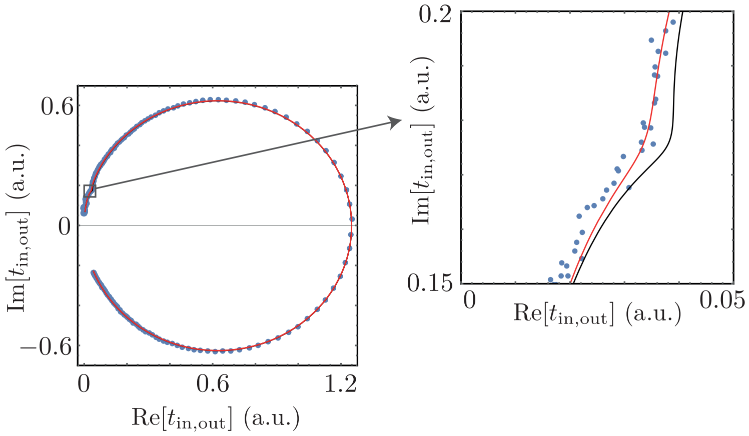


Figure S2: **Calibration of the excitation probability at equilibrium a)** Blue dots: Fresnel plane representation of the transmission of the cavity when probed in continuous wave with the qubit at thermal equilibrium. The cavity mode is probed from 7.83 to 7.87 GHz. The probe power is weak enough so that the occupation of the cavity is $\leqslant 1$ photon in the stationary state (no visible anharmonicity of the cavity). Red line: fit in $p_{\mathrm{eq}}$. The transmission coefficient is fitted by a double Lorentzian, respectively centered in $f_c$ and $f_c - \chi$ and each with the same width $\kappa_{\mathrm{tot}}$ given in Sec. I A and the same scaling factor. The relative weight $p_{\mathrm{eq}}/(1-p_{\mathrm{eq}})$ is adjusted with $p_{\mathrm{eq}} = 0.7$ % on the red line. Black line: calculated transmission coefficient for the upper bound on $p_{\mathrm{eq,max}} = 1$ %. **b)** Zoom of a for probe frequency around $f_c - \chi$.

The qubit state is measured independently using the cavity resonance frequency as a probe. In order to get a single shot measurement, one may use the so-called regime of "high power readout" [3]. However, in this particular run of the experiment, the coherence time of the qubit was degraded for tens of milliseconds after using high power readout. This could be due to the creation of quasi particles, whose relaxation was recently shown to occur on such long timescales [4, 5]. Note that in a previous run, this relaxation time-scale was several orders of magnitude lower. It

increased after an unwanted warm-up of the refrigerator just above superconducting aluminum critical temperature. This is consistent with recent observation of quasi-particle induced noise suppression due to vortices in aluminum thin films [5, 6]. These vortices are created when cooling down the sample under constant magnetic field and act as quasi-particle traps, and these conditions might have not been the same for the present cool down.

Therefore, in this run of the experiment, the pulse power was chosen as a tradeoff between a good readout fidelity and short repetition rate of the experiment $T_{\text{repet}} = 80\ \mu$s. The qubit state is projectively measured by applying a $2\mu$s-long pulse at $f_{\text{readout}} = 7.8534$ GHz close to the cavity resonance frequency. Integrating the transmitted signal, one gets a direct measurement of the qubit state (see Eq. (S1)).

Once the readout power was set, the pulse frequency was empirically adjusted to maximize the discrimination between the two qubit states. Note that at the chosen power, the cavity resonance frequency is shifted due to the anharmonicity of the cavity mode inherited from its coupling with the qubit. This frequency thus corresponds to the maximum transmission of the cavity when the qubit is in $|g\rangle$.
For a given integrated amplitude of the transmitted signal $\alpha$, we then define the detection event $D =$ "$|a| < T$", where $a$ is the integrated signal amplitude and $T$ is an arbitrary detection threshold. Ideally, we would like that $D$ is always true if the qubit is in $|g\rangle$ and always false if it is in $|e\rangle$. The readout fidelities are then defined as $f_g = P(\overline{D}|g)$ and $f_e = P(D|e)$ ($1 - f_g$ and $1 - f_e$ are respectively the false positive and false negative probabilities of the detection). Those are calibrated by measuring $P(D)$ when the qubit is at thermal equilibrium or after a $\pi$-pulse. Indeed,

$$\begin{cases} P(D) = (1-p_{\text{eq}})(1-f_g) + p_{\text{eq}} f_e & \text{at equilibrium} \\ P(D) = p_{\text{eq}}(1-f_g) + (1-p_{\text{eq}}) f_e & \text{after a } \pi-\text{pulse} \end{cases}, \tag{S2}$$

where $p_{\text{eq}} = 0.7$ % was extracted from the spectroscopy of the cavity at low power (see Fig. S2).
For the chosen detection threshold, we found $f_g = f_e = 0.85$. Thus, even without a quantum limited amplifier at the cavity frequency, we can discriminate between $|g\rangle$ and $|e\rangle$ with 85% fidelity in a single-shot.

For ensemble averages such as the one performed during the tomography of the qubit state in Sec. III, the measured value of $z_{\text{tomo}}$ is then found by solving, similarly to Eq. (S2),

$$P(D) = \frac{1 - z_{\text{tomo}}}{2}(1 - f_g) + \frac{1 + z_{\text{tomo}}}{2} f_e. \tag{S3}$$

Thus, when the detection probability on an ensemble of realizations is $P(D)$, $z_{\text{tomo}} = \frac{f_g - f_e - 1 + 2P(D)}{f_g + f_e - 1}$.
This formula holds for $\sigma_x$ and $\sigma_y$ measurement, with the same fidelities. Indeed, imperfections of the fast $\pi/2$ rotation pulses applied before the readout to map the $x$ or $y$ axis onto the $z$ axis and decoherence during these pulses can be neglected.

To estimate the length $2\Delta\alpha_{\text{tomo}}$ ($\alpha = x, y, z$) of the error bars in Fig. 3, we first compute the statistical uncertainty on the measured detection probability $\Delta D = \sqrt{\frac{P(D)\big(1-P(D)\big)}{N}}$, where $N$ is the number of realizations in the ensemble. We then scale this value taking into account the finite detection fidelity as $\Delta\alpha_{\text{tomo}} = \Delta\alpha_{\text{tomo}} = \frac{2}{f_g + f_e - 1}\Delta D$.

## II. FROM RAW DATA TO TRAJECTORIES

### A. From raw data to measurement records

The fluorescence field on the output line is amplified by a low-noise detection setup, down-converted to $f_h = 100$ MHz and then digitized and numerically demodulated, so that the sampling step is $\mathrm{d}t = 200$ ns. The data that is recorded thus corresponds to discrete times $k\mathrm{d}t$.

The JPC that is used as a pre-amplifier has a gain $G \simeq 25$dB. Using a vector network analyzer on the reflection probe, we estimate its amplification bandwidth to be $2\pi \times 3$ MHz $\gg \gamma_1$, which limits the bandwidth of the whole detection setup. The fluorescence signal is only slightly distorted by this finite bandwidth. After integrating the demodulated signal from $t$ to $t + \mathrm{d}t$, which defines the records $\mathrm{d}\tilde{I}_t$ and $\mathrm{d}\tilde{Q}_t$, the effect can be modeled as a first-order low-pass filter. Its time constant $\tau_c$ can be precisely calibrated, along with the scaling factor $\beta$ that allows to normalize the variance of $\mathrm{d}I$ and $\mathrm{d}Q$ to $\mathrm{d}t$, and it can then be corrected for. Indeed, considering two successive time steps $t - \mathrm{d}t$ and $t$, the digitized records are given at first order by

$$\begin{cases} \mathrm{d}\tilde{I}_t &= \lambda\beta \mathrm{d}I_t + (1-\lambda)\mathrm{d}\tilde{I}_{t-\mathrm{dt}} \\ \mathrm{d}\tilde{Q}_t &= \lambda\beta \mathrm{d}Q_t + (1-\lambda)\mathrm{d}\tilde{Q}_{t-\mathrm{dt}}, \end{cases} \tag{S4}$$

where $\lambda$ is defined by $\tau_c = -\frac{\mathrm{d}t}{\log 1-\lambda}$ and $\{\mathrm{d}I_t, \mathrm{d}Q_t\}$ would be the records for a setup with an infinite bandwidth. We then consider records much longer than $\tau_c$ and for a qubit prepared in $|g\rangle$ so that there is no signal on average. In that case, $\mathrm{d}I_t = \mathrm{d}W_t$ at all times $t$, where $W$ is a Wiener process. By definition, $\mathbb{E}[\mathrm{d}W_t \mathrm{d}W_{t'}] = \delta_{t,t'}\mathrm{d}t$. Then, for $t \gg \tau_c$,

$$\begin{aligned}\mathbb{E}[\mathrm{d}\tilde{I}_t^2] &= \mathbb{E}[(\beta\lambda \sum_{k=0}^{t/\mathrm{d}t}(1-\lambda)^k \mathrm{d}I_{t-k\mathrm{d}t})^2] \\ &= \beta^2\lambda^2 \sum_{k=0}^{t/\mathrm{d}t}(1-\lambda)^{2k}\mathrm{d}t \\ &= \tfrac{\beta^2\lambda\mathrm{d}t}{2-\lambda}\left(1-(1-\lambda)^{2t/\mathrm{d}t+1}\right) \\ &= \tfrac{\beta^2\lambda\mathrm{d}t}{2-\lambda},\end{aligned} \tag{S5}$$

and similarly,

$$\mathbb{E}[\mathrm{d}\tilde{I}_t \mathrm{d}\tilde{I}_{t-\mathrm{d}t}] = \frac{\beta^2\lambda(1-\lambda)\mathrm{d}t}{2-\lambda}. \tag{S6}$$

We can then extract the value of $\beta$ and $\lambda$. We find $\tau_c = 100$ ns, which is consistent with the detection bandwidth estimated through spectroscopy measurements. We then recover the measurement records before any amplification or filtering

$$\begin{cases}\mathrm{d}I_t &= \frac{\mathrm{d}\tilde{I}_t + (\lambda-1)\mathrm{d}\tilde{I}_{t-\mathrm{d}t}}{\lambda\beta} \\ \mathrm{d}Q_t &= \frac{\mathrm{d}\tilde{Q}_t + (\lambda-1)\mathrm{d}\tilde{Q}_{t-\mathrm{d}t}}{\lambda\beta}\end{cases}. \tag{S7}$$

On Fig. S3, are represented the raw digitized records (in black) corresponding to the corrected records presented

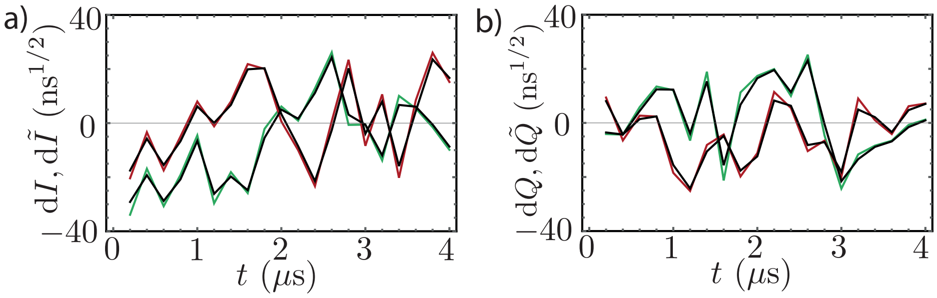


Figure S3: **Raw data versus records corrected for detection finite bandwidth.** The black lines represent the raw digitized signal $\mathrm{d}\tilde{I}_t, \mathrm{d}\tilde{Q}_t$ from which the measurement records $\mathrm{d}I_t, \mathrm{d}Q_t$ represented in Fig. 2 are extracted. These corrected records are represented by red and green lines (same color code as in Fig. 2) and only slightly differ from the raw data which is smoothed due to the finite bandwidth of the measurement setup.

on Fig. 2a (represented here with the same color code). Once rescaled, the raw data, which is altered by the finite bandwidth of the detection setup, only slightly differs from the measurement records that were used to reconstruct the trajectories.

### B. Discrete time Stochastic Master Equation

The trajectories are reconstructed using a discrete time formulation of the Stochastic Master Equation (2) that is better suited for finite sampling step $\mathrm{d}t$ [7]. It reads

$$\rho_{t+\mathrm{d}t} = \frac{M_t\rho_t M_t^\dagger + (1-\eta)\gamma_1\sigma_-\rho_t\sigma_+\mathrm{d}t + \frac{\gamma_\phi}{2}\sigma_Z\rho_t\sigma_Z\mathrm{d}t}{\mathrm{Tr}[M_t\rho_t M_t^\dagger + (1-\eta)\gamma_1\sigma_-\rho_t\sigma_+\mathrm{d}t + \frac{\gamma_\phi}{2}\sigma_Z\rho_t\sigma_Z\mathrm{d}t]}, \tag{S8}$$

where the pseudo Kraus operator $M_t$ depends on the measurement record as

$$M_t = \mathbf{1} - (iH + \frac{\gamma_1}{2}\sigma_+\sigma_- + \frac{\gamma_\phi}{4}\mathbf{1})\mathrm{d}t + \sqrt{\frac{\eta\gamma_1}{2}}\sigma_-(\mathrm{d}I_t + i\mathrm{d}Q_t). \tag{S9}$$

The trajectories are then constructed step by step from the measurement records.

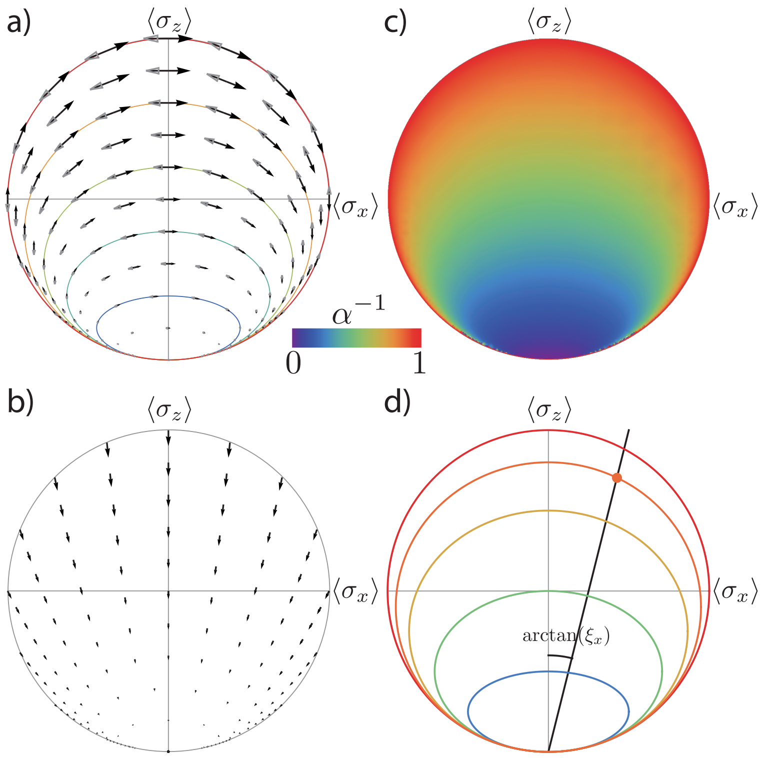


Figure S4: **Representation of measurement back action and decoherence. a)** Representation of the typical step in the diffusion of the Bloch vector, in the $\langle\sigma_y\rangle = 0$ plane, due to the stochastic term in $\mathrm{d}W_{I,t}$ of Eq. (S10) during a time $\mathrm{d}t = 200$ ns with an efficiency $\eta = 0.24$. Each double sided arrow represents a possible increase of the Bloch vector. The middle of the arrow sits at the initial Bloch vector at time $t$ and the black (respectively gray) tip of the arrow indicates the displacement of the Bloch vector due to the stochastic terms in Eq. (S10), when the value of $\mathrm{d}W_{I,t}$ is $\sqrt{\mathrm{d}t}$ (resp. $-\sqrt{\mathrm{d}t}$). The colored ellipses are solutions of Eq. (4) and are tangent to the diffusion step. **b)** In a similar representation is shown the deterministic average effect of relaxation at a rate $\gamma_1 = (4\ \mu\mathrm{s})^{-1}$ during the same time step $\mathrm{d}t$ following the terms in $\mathrm{d}t$ of Eq. (S10). **c)** Colorplot of the parameter $\alpha$ defined in Eq. (3) in the Bloch sphere representation. **d)** Geometric interpretation of the parameter $\xi_x$ that is related to integrals of the measured quadratures (see Eq. (S16)).

## III. MEASUREMENT BACKACTION

### A. Backaction of heterodyne measurement

The stochastic master equation (2) in the article does not express clearly the effect of measurement backaction on the quantum state of the qubit. Looking at the diffusion step of the Bloch vector is a good way to understand this effect. This was already done almost 20 years ago by Hofmann et al. [8] in a slightly different language. Equation (2) can be expressed in Bloch coordinates as

$$\left\{\begin{array}{lcl} \mathrm{d}x &=& -(\frac{\gamma_1}{2}+\gamma_\phi)x\mathrm{d}t + \sqrt{\frac{\eta\gamma_1}{2}}\left((z+1-x^2)\mathrm{d}W_{I,t} - xy\mathrm{d}W_{Q,t}\right) \\ \mathrm{d}y &=& -(\frac{\gamma_1}{2}+\gamma_\phi)y\mathrm{d}t + \sqrt{\frac{\eta\gamma_1}{2}}\left((z+1-y^2)\mathrm{d}W_{Q,t} - xy\mathrm{d}W_{I,t}\right) \\ \mathrm{d}z &=& -\gamma_1(z+1)\mathrm{d}t - \sqrt{\frac{\eta\gamma_1}{2}}(z+1)\left(x\mathrm{d}W_{I,t} + y\mathrm{d}W_{Q,t}\right) \end{array}\right. . \quad \text{(S10)}$$

One can distinguish two separate contributions in these equations. The first one is a deterministic evolution in $\mathrm{d}t$ coming from the average decay and captured by the Lindblad terms in Eq. (2). The second one is a stochastic term in $\mathrm{d}W$ coming from the zero point fluctuations in heterodyne measurement. In the experiment, the time steps were chosen to be $\mathrm{d}t = 200$ ns, and $|\mathrm{d}W|$ is typically given by $\sqrt{\mathrm{d}t}$. These contributions are captured in Figs. S4a and S4b. Up to a rotation in the Bloch sphere, the same figure captures the dual effect of measuring $\mathrm{d}Q$.

This figure clarifies the kind of measurement records that are required to observe an increase of excitation probability during decay. Starting in $|+x\rangle$ as in Fig. 2a,b, negative values of $\mathrm{d}W_{I,t}$ in the beginning lead to an increase of $z$ for the Bloch vector. This is why the trajectory in green of Fig. 2b corresponds to a measurement record which starts negative in $\mathrm{d}I$.

### B. Deterministic surface spanned by the trajectories

In the case $\gamma_\phi = 0$, it is possible to convert Eq. (S10) in cylindrical coordinates $\{x, y\} \to \{r\cos(\theta), r\sin(\theta)\}$, which then reads

$$\left\{\begin{array}{lll} \mathrm{d}r & = & \frac{\gamma_1}{2}\left(\frac{\eta(1+z)^2}{2r} - r\right)\mathrm{d}t + \sqrt{\frac{\eta\gamma_1}{2}}(z+1-r^2)\mathrm{d}W_{r,t} \\ \mathrm{d}z & = & -\gamma_1(z+1)\mathrm{d}t - \sqrt{\frac{\eta\gamma_1}{2}}(z+1)r\mathrm{d}W_{r,t} \\ \mathrm{d}\theta & = & \sqrt{\frac{\eta\gamma_1}{2}}\frac{z+1}{r}\mathrm{d}W_{\theta,t} \end{array}\right. . \tag{S11}$$

Here, $\mathrm{d}W_{r,t} = \cos\theta\mathrm{d}W_{I,t} + \sin\theta\mathrm{d}W_{Q,t}$ and $\mathrm{d}W_{\theta,t} = -\sin\theta\mathrm{d}W_{I,t} + \cos\theta\mathrm{d}W_{Q,t}$ are obtained by rotation in the Bloch sphere so that their variance is still $\mathrm{d}t$ and they are uncorralated.

Let us now derive the dynamics of the parameter $\alpha$ in Eq. (3)

$$\alpha = \frac{2}{1+z} - \frac{r^2}{(1+z)^2}. \tag{S12}$$

A graphical representation of $\alpha$ is given in Fig. S4c. Then, from the above equation, and after some calculation following the Itô rules, one gets

$$\mathrm{d}\alpha = (\alpha - \eta)\gamma\mathrm{d}t, \tag{S13}$$

which leads to Eq. (4).

### C. Integrable quantities for heterodyne measurement of fluorescence

In Sec. IV, we have defined the quantities $\xi_x = \frac{x}{z+1}$ and $\xi_y = \frac{y}{z+1}$, whose geometric interpretation in the Bloch sphere is captured by Fig. S4d. Starting from Eq. (S10), neglecting $\gamma_\phi$ and applying Itô rules, we find that

$$\begin{array}{lll} \mathrm{d}\xi_x & = & \frac{\gamma_1}{2}\xi_x\mathrm{d}t + \sqrt{\frac{\eta\gamma_1}{2}}\mathrm{d}W_t + \frac{\eta\gamma_1}{2}x\mathrm{d}t \\ & = & \frac{\gamma_1}{2}\xi_x\mathrm{d}t + \sqrt{\frac{\eta\gamma_1}{2}}\mathrm{d}I_t. \end{array} \tag{S14}$$

This leads to

$$\mathrm{d}\left(\xi_x e^{-\gamma_1 t/2}\right) = \sqrt{\frac{\eta\gamma_1}{2}}e^{-\gamma_1 t/2}\mathrm{d}I_t. \tag{S15}$$

Integrating this equation between times 0 and $T$, on a single trajectory we get the equality of Eq. (5)

$$e^{-\frac{\gamma_1}{2}T}\frac{x(T)}{z(T)+1} - \frac{x(0)}{z(0)+1} = \sqrt{\frac{\eta\gamma_1}{2}}\int_0^T e^{-\frac{\gamma_1}{2}t}\mathrm{d}I_t \overset{\mathrm{def}}{\equiv} \sqrt{\frac{\eta\gamma_1}{2}}m_I, \tag{S16}$$

where we have defined the integrated quantity $m_I$. We now validate this equality on $\xi_x(T)$ experimentally, similarly to what is done in Fig. 3 for the predicted Bloch coordinates at $T$. Let us note that, contrary to $m_I$, $x(T) = \mathrm{Tr}[\rho_T\sigma_X]$, $z(T) = \mathrm{Tr}[\rho_T\sigma_Z]$ or $\xi_x(T)$ are not directly measurable on a single experiment. Yet, when considering a great number $N$ of trajectories from the same initial state and giving the same measured $m_I$, if we were to reconstruct the whole trajectory, we would find N different $\rho_k$'s with

$$\text{for all } k, \sqrt{\frac{\eta\gamma_1}{2}}m_I = e^{-\frac{\gamma_1}{2}T}\frac{\mathrm{Tr}[\rho_k\sigma_X]}{\mathrm{Tr}[\rho_k\sigma_Z]+1} - \frac{x(0)}{z(0)+1}, \tag{S17}$$

so that averaging both sides of the equation over $k$ and using the mathematical property that if for all $k$, $\frac{a_k}{b_k} = \epsilon$, then $\frac{\sum_k a_k}{\sum_k b_k} = \epsilon$, we find that

$$\begin{array}{lll} \sqrt{\frac{\eta\gamma_1}{2}}m_I & = & e^{-\frac{\gamma_1}{2}T}\dfrac{\frac{1}{N}\sum_k \mathrm{Tr}[\rho_k\sigma_X]}{\frac{1}{N}\sum_k \mathrm{Tr}[\rho_k\sigma_Z]+1} - \dfrac{x(0)}{z(0)+1} \\ & = & e^{-\frac{\gamma_1}{2}T}\dfrac{\mathrm{Tr}[\overline{\rho}^{m_I}\sigma_X]}{\mathrm{Tr}[\overline{\rho}^{m_I}\sigma_Z]+1} - \dfrac{x(0)}{z(0)+1}. \end{array} \tag{S18}$$

Here, $\overline{\rho}^{m_I}$ is the density matrix corresponding to the statistical mixture of all final states of the realizations of the experiment that yielded the same $m_I$. Thus, $\mathrm{Tr}[\overline{\rho}^{m_I}\sigma_\alpha]$ $(\alpha = x, z)$ corresponds to the measured average value $\alpha_{\mathrm{tomo}}$ on this sub ensemble of experiments.

Similarly, defining $m_Q = \int_0^T e^{-\frac{\gamma_1}{2}t}\mathrm{d}Q$, when selecting experiments giving the same $m_Q$, we have

$$e^{-\frac{\gamma_1}{2}T}\frac{\mathrm{Tr}[\overline{\rho}^{m_I}\sigma_Y]}{\mathrm{Tr}[\overline{\rho}^{m_I}\sigma_Z]+1} = \sqrt{\frac{\eta\gamma_1}{2}}m_Q + \frac{y(0)}{z(0)+1}. \tag{S19}$$

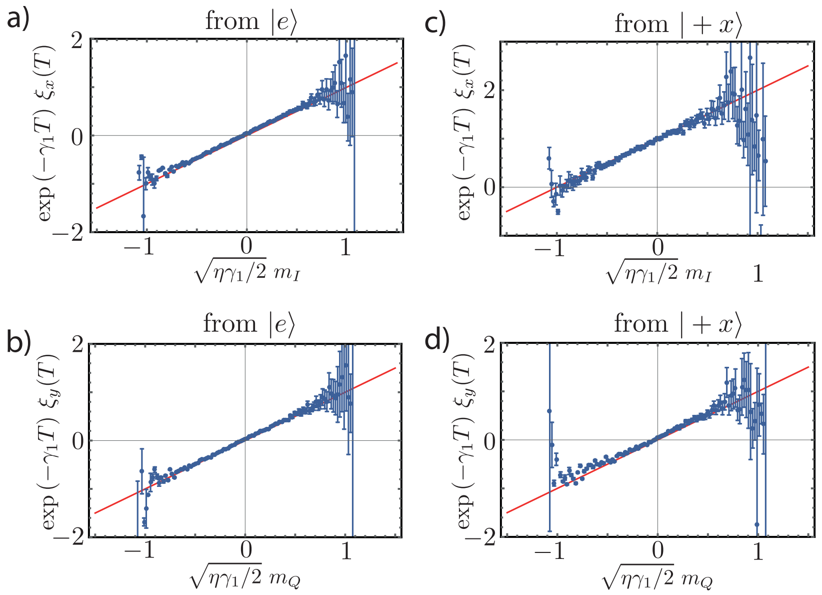


Figure S5: **a)** For a qubit prepared in $|e\rangle$, the fluorescence signal is integrated for $T = 4\ \mu$s with a decreasing exponential weight (see Eq. (S16)). Experiments with the same resulting integral $m_I$ are binned together and we plot here the measured mean value per bin of $\xi_x = \frac{x}{z+1}$ given by the final readout as a function of $m_I$. Error bars correspond to statistical errors due to the limited number of experiments per value of $m_I$. The red line corresponds to the linear function $\sqrt{\frac{\eta\gamma_1}{2}}m_I + \xi_x(0)$. **b)** Same plot for $m_Q$. **c,d)** Same plots in the case where the qubit starts in $|+x\rangle$.

The validity of these equalities can be checked on Fig. S5a,b, for trajectories starting in $|+x\rangle$ and recording the fluorescence field for $T = 4\ \mu$s. We sorted the trajectories according to the value of $m_I$ and placed them into 111 bins. For each bin $i$ and using the trajectories for which we measured $\sigma_z$ (resp. $\sigma_x$) at $T$, we compute the average value $z_{\mathrm{tomo}}(i)$ (resp. $x_{\mathrm{tomo}}(i)$). Plotting $\frac{x_{\mathrm{tomo}}(i)}{z_{\mathrm{tomo}}(i)+1}$ as a function of $m_I(i)$, a linear dependence clearly appears and it matches the expected law in Eq. (S16). Symmetrically, when sorting the trajectories according to the values of $m_Q$ and placing them into the bins $j$, the same slope appears when plotting $\frac{y_{\mathrm{tomo}}(j)}{z_{\mathrm{tomo}}(j)+1}$ as a function of $m_Q(j)$. The agreement is also good for the trajectories starting in $|e\rangle$ (Fig. S5c,d) and for all trajectory duration $T$.

## IV. STATISTICS OF QUANTUM TRAJECTORIES

In the main text, the representation of the distributions of states in Fig. 4 gives an imprecise idea of the thickness of the shell below the surface of the spheroid characterized by Eq. (5). In Fig. S6 are shown cuts of these distributions in the plane $y = 0$ of the Bloch sphere (strictly speaking, we used the volume defined by $0 \leq y < 0.04$. The spread of the distribution beyond the spheroid surface becomes apparent. It is here due to the finite pure dephasing time $\gamma_\phi^{-1} = 35\ \mu$s. As expected, the effect of dephasing is stronger and the departure from the spheroid is larger for trajectories starting in $|+x\rangle$ than in $|e\rangle$. A movie of the evolution of the distribution of states can be found as a supplementary material for each initial state.

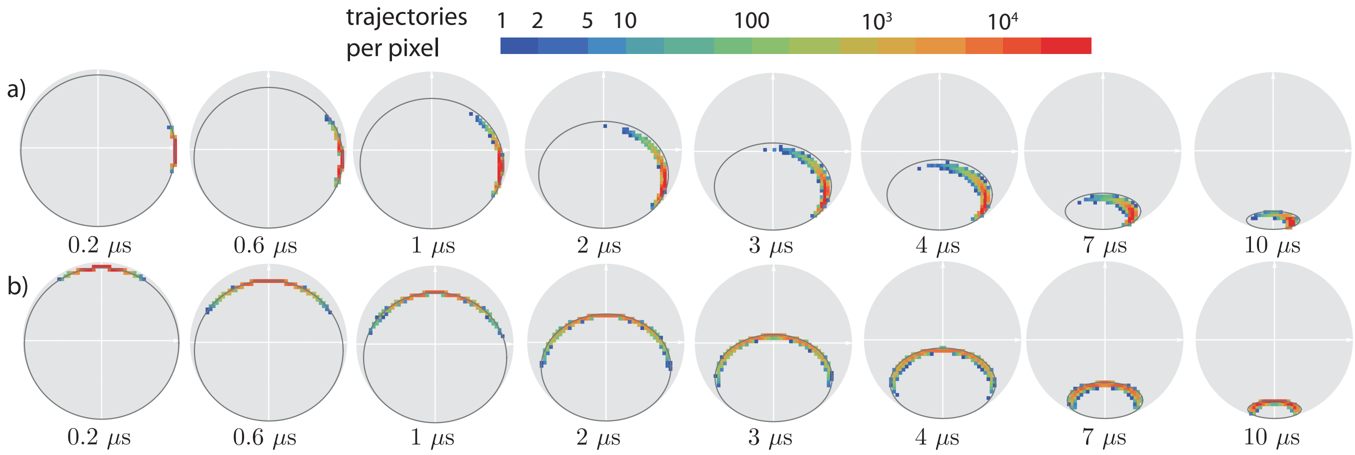


Figure S6: **Statistics of quantum trajectories.** Same distributions of the qubit states along 10 $\mu$s-long trajectories for a qubit initially in $|+x\rangle$ (**a**) and $|e\rangle$ (**b**) as in Fig. 4. Each panel represents a cut of the Bloch sphere at $\langle\sigma_y\rangle = 0$. The number of trajectories reaching each pixel of side 0.04 is encoded in color. White arrows go from $-1$ to $+1$ along $\sigma_{x,z}$ and the Bloch sphere is colored in gray. The intersection between the spheroid characterized by Eq. (5) and the plane $y = 0$ is also shown.


[1] H. Paik, D. I. Schuster, L. S. Bishop, G. Kirchmair, G. Catelani, a. P. Sears, B. R. Johnson, M. J. Reagor, L. Frunzio, L. I. Glazman, S. M. Girvin, M. H. Devoret and R. J. Schoelkopf. Observation of High Coherence in Josephson Junction Qubits Measured in a Three-Dimensional Circuit QED Architecture. *Physical Review Letters* **107**, 240501 (2011).

[2] N. Roch, E. Flurin, F. Nguyen, P. Morfin, P. Campagne-Ibarcq, M. H. Devoret and B. Huard. Widely Tunable, Nondegenerate Three-Wave Mixing Microwave Device Operating near the Quantum Limit. *Physical Review Letters* **108**, 147701 (2012).

[3] M. Reed, L. DiCarlo, B. Johnson, L. Sun, D. Schuster, L. Frunzio and R. Schoelkopf. High-fidelity readout in circuit quantum electrodynamics using the Jaynes-Cummings nonlinearity. *Physical review letters* **105**, 173601 (2010).

[4] D. Ristè, C. Bultink, M. Tiggelman, R. Schouten, K. Lehnert and L. DiCarlo. Millisecond charge-parity fluctuations and induced decoherence in a superconducting transmon qubit. *Nature communications* **4**, 1913 (2013).

[5] U. Vool, I. M. Pop, K. Sliwa, B. Abdo, C. Wang, T. Brecht, Y. Y. Gao, S. Shankar, M. Hatridge, G. Catelani *et al.* Non-Poissonian quantum jumps of a fluxonium qubit due to quasiparticle excitations. *Physical review letters* **113**, 247001 (2014).

[6] I. Nsanzineza and B. L. T. Plourde. Trapping a single vortex and reducing quasiparticles in a superconducting resonator. *Phys. Rev. Lett.* **113**, 117002 (2014).

[7] P. Rouchon and J. F. Ralph. Efficient Quantum Filtering for Quantum Feedback Control. *arXiv preprint arXiv:1410.5345* (2014).

[8] H. F. Hofmann, O. Hess and G. Mahler. Quantum control of atomic systems by time-resolved homodyne detection of spontaneous emission. *Phys. Rev. A* **57**, 5 (1998).
